# Supplementary material for: The fourth- and fifth-order virial coefficients from weak-coupling to unitarity
Source: arXiv:2004.08685 ancillary file (2020-04-18)
Supplement: Supplementary file 1 [file supplemental-materials-prl.pdf]

# Supplemental Material for
# The fourth- and fifth-order virial coefficients from weak-coupling to unitarity.

Y. Hou[1] and J. E. Drut[1]

[1]*Department of Physics and Astronomy, University of North Carolina, Chapel Hill, North Carolina 27599, USA*

(Dated: April 18, 2020)

In these supplemental materials, we show the details of the formalism underlying our automated algebra method, together with a discussion of its computational costs and scalability. We also present intermediate results using the two different types of renormalizations mentioned in the main text, which agree within error bars, and explain how the continuum-limit extrapolations are made to obtain those error bars. The estimates for $\Delta b_n$ and $\Delta b_{mj}$ for $n = 3, 4, 5$ and $m + j = n$ from the weakly-coupling to the unitary limit are summarized in a reference table. Lastly, we show how our results modify the virial expansion for several quantities, comparing with experimental data and other theoretical approaches where available.

## CONTENTS

I. Formalism and Automated Algebra Method 1

II. Renormalization 3

III. Extrapolation to the large-$k$ limit and resulting uncertainty 4

IV. Comparison of $\Delta b_2$ and transfer-matrix renormalization procedures. 6

V. Derivation of Polarized Virial Coefficients $\Delta b_{mj}$ 7

VI. Applications 7
- A. Tan's contact of spin-balanced system 8
- B. Tan's contact of spin-imbalanced system 9
- C. Magnetization 10

VII. Resummation techniques 11

References 11

## I. FORMALISM AND AUTOMATED ALGEBRA METHOD

Equation (11) in the main text shows the Trotter-Suzuki factorization of the Boltzmann weight, which yields an expression for the canonical partition function $Q_N$, in momentum representation, given by

$$Q_{MJ} = \mathrm{Tr}\left(\mathrm{e}^{-\beta \hat{H}}\right) \simeq \sum_{|\mathbf{P}\rangle} \langle \boldsymbol{P}| \left(e^{-\beta \hat{T}/(2k)} e^{-\beta \hat{V}/k} e^{-\beta \hat{T}/(2k)}\right)^k |\boldsymbol{P}\rangle \,, \tag{1}$$

where $\hat{H} = \hat{T} + \hat{V}$ and we use the abbreviation $|\boldsymbol{P}\rangle = |p_1 \cdots p_M; p_{M+1} \cdots p_{M+J}\rangle$. Here, the subscript 1 to $M$ corresponds to the $M$ spin-$\uparrow$ particles and $M+1$ to $M+J$ corresponds to the $J$ spin-$\downarrow$ particles. Inserting $k$ complete sets of states $\sum |\boldsymbol{P}\rangle\langle\boldsymbol{P}|$ in between the kinetic- and potential-energy operators, and using the fact that the kinetic-energy operator $\hat{T}$ is diagonal in momentum space, we obtain

$$Q_{MJ} = \sum_{|\mathbf{P}\rangle} \mathrm{e}^{-\frac{\beta}{2m}(\boldsymbol{P_1}^2 + \boldsymbol{P_2}^2 + \cdots + \boldsymbol{P_k}^2)} \langle \boldsymbol{P_1}|\mathrm{e}^{-\beta \hat{V}/k}|\boldsymbol{P_2}\rangle \, \langle \boldsymbol{P_2}|\mathrm{e}^{-\beta \hat{V}/k}|\boldsymbol{P_3}\rangle \cdots \langle \boldsymbol{P_k}|\mathrm{e}^{-\beta \hat{V}/k}|\boldsymbol{P_1}\rangle \,, \tag{2}$$

where the cyclic property of trace is used and $\boldsymbol{P_1^2} = p_1^2 + p_2^2 \cdots + p_{M+J}^2$. To evaluate the potential-energy factors, another round of $k$ complete sets of states is inserted, now in coordinate space, to obtain

$$\begin{aligned} Q_{MJ} = \sum_{|\mathbf{P}\rangle,|\mathbf{X}\rangle} \mathrm{e}^{-\frac{\beta}{2m}(\boldsymbol{P_1^2}+\boldsymbol{P_2^2}+\cdots+\boldsymbol{P_k^2})} \langle \boldsymbol{P_1}|\boldsymbol{X_1}\rangle \langle \boldsymbol{X_1}|\boldsymbol{P_2}\rangle \langle \boldsymbol{P_2}|\boldsymbol{X_2}\rangle \langle \boldsymbol{X_2}|\boldsymbol{P_3}\rangle \cdots \langle \boldsymbol{P_k}|\boldsymbol{X_k}\rangle \langle \boldsymbol{X_k}|\boldsymbol{P_1}\rangle \\ \times \langle \boldsymbol{X_1}|\mathrm{e}^{-\beta\hat{V}/k}|\boldsymbol{X_1}\rangle \ \langle \boldsymbol{X_2}|\mathrm{e}^{-\beta\hat{V}/k}|\boldsymbol{X_2}\rangle \cdots \ \langle \boldsymbol{X_k}|\mathrm{e}^{-\beta\hat{V}/k}|\boldsymbol{X_k}\rangle \,, \end{aligned} \tag{3}$$

where we have used the fact that $\hat{V}$ is diagonal in coordinate space, since $\hat{V} = -g\sum_{\mathbf{x}} \hat{n}_\uparrow(\mathbf{x})\hat{n}_\downarrow(\mathbf{x})$. In the above equation, $\langle \boldsymbol{X}|\boldsymbol{P}\rangle$ is a Slater determinant which, written explicitly using a plane-wave basis of single-particle states, is

$$\begin{aligned} \langle \boldsymbol{X}|\boldsymbol{P}\rangle &= \sum_{\epsilon} \epsilon_{i_1 i_2\cdots i_M}\epsilon_{j_1 j_2\cdots j_J} \langle x_1|p_{i_1}\rangle \langle x_2|p_{i_2}\rangle \cdots \langle x_M|p_{i_M}\rangle \langle x_{M+1}|p_{j_1}\rangle \langle x_{M+2}|p_{j_2}\rangle \cdots \langle x_{J+M}|p_{j_J}\rangle \\ &= \sum_{\epsilon} \epsilon_{i_1 i_2\cdots i_M}\epsilon_{j_1 j_2\cdots j_J} \mathrm{e}^{ix_1 p_{i_1}} \mathrm{e}^{ix_2 p_{i_2}} \cdots \mathrm{e}^{ix_M p_{i_M}} \mathrm{e}^{ix_{M+1} p_{j_1}} \mathrm{e}^{ix_{M+2} p_{j_2}} \cdots \mathrm{e}^{ix_{M+J} p_{j_J}} \,, \end{aligned} \tag{4}$$

where $\epsilon$ is the Levi-Civita tensor [Note that we have omitted volume factors as well as $M!$ and $J!$ factors to simplify the presentation]. To evaluate the matrix elements of the potential-energy factor $\mathrm{e}^{-\beta\hat{V}/k}$, we use the identity

$$\begin{aligned} \mathrm{e}^{-\beta\hat{V}/k} &= \prod_{\mathbf{x}} \mathrm{e}^{\beta g \hat{n}_\uparrow(\mathbf{x})\hat{n}_\downarrow(\mathbf{x})/k} = \prod_{\mathbf{x}} [1 + C\hat{n}_\uparrow(\mathbf{x})\hat{n}_\downarrow(\mathbf{x})] \\ &= \mathbf{1} + C\sum_{\mathbf{z}} \hat{n}_\uparrow(\mathbf{z})\hat{n}_\downarrow(\mathbf{z}) + \frac{C^2}{2!}{\sum_{\mathbf{z}\mathbf{z}'}}' \hat{n}_\uparrow(\mathbf{z})\hat{n}_\downarrow(\mathbf{z})\hat{n}_\uparrow(\mathbf{z}')\hat{n}_\downarrow(\mathbf{z}') + \cdots \,, \end{aligned} \tag{5}$$

where $C = e^{\beta g/k} - 1$, the primed sum indicates the constraint that $\mathbf{z} \neq \mathbf{z}'$, and we used the fermionic property $\hat{n}_\sigma^2 = \hat{n}_\sigma$. The matrix element is then evaluated as

$$\begin{aligned} \langle \boldsymbol{X}|\mathrm{e}^{-\beta\hat{V}/k}|\boldsymbol{X}\rangle = \mathbf{1} &+ C\sum_{\mathbf{z}}\sum_{i=1}^{M}\sum_{j=M+1}^{M+J} \delta(x_i - \mathbf{z})\delta(x_j - \mathbf{z}) \\ &+ \frac{C^2}{2!}{\sum_{\mathbf{z}\mathbf{z}'}}'\sum_{i=1}^{M}\sum_{j=M+1}^{M+J} \delta(x_i - \mathbf{z})\delta(x_j - \mathbf{z}) \sum_{i'=1}^{M}\sum_{j'=M+1}^{M+J} \delta(x_i' - \mathbf{z}')\delta(x_j' - \mathbf{z}') + \cdots \,. \end{aligned} \tag{6}$$

The series is finite and is cut off at order $\min(M, J)$ due to the constraint $\mathbf{z} \neq \mathbf{z}' \neq \cdots$. Further simplification is possible by considering the identical particle symmetry, resulting in

$$\langle \boldsymbol{X}|\mathrm{e}^{-\beta\hat{V}/k}|\boldsymbol{X}\rangle = \mathbf{1} + C \cdot M \cdot J\delta(x_1 - x_{M+1}) + \frac{C^2}{2!} \cdot {}^{M}P_2 \cdot {}^{J}P_2 \delta(x_1 - x_{M+1})\delta(x_2 - x_{M+2}) + \cdots \,, \tag{7}$$

where ${}^{n}P_k = \frac{n!}{(n-k)!}$ is the permutation number. Expanding all potential-energy terms and grouping them according to the power of $C$, we obtain the canonical partition function $Q_N$ as a polynomial in $C$:

$$\begin{aligned} Q_{MJ} = \sum_{|\mathbf{P}\rangle,|\mathbf{X}\rangle} \mathrm{e}^{-\frac{\beta}{2m}(\boldsymbol{P_1^2}+\boldsymbol{P_2^2}+\cdots+\boldsymbol{P_k^2})} \langle \boldsymbol{P_1}|\boldsymbol{X_1}\rangle \langle \boldsymbol{X_1}|\boldsymbol{P_2}\rangle \langle \boldsymbol{P_2}|\boldsymbol{X_2}\rangle \langle \boldsymbol{X_2}|\boldsymbol{P_3}\rangle \cdots \langle \boldsymbol{P_k}|\boldsymbol{X_k}\rangle \langle \boldsymbol{X_k}|\boldsymbol{P_1}\rangle \\ \times \Big(1 + Cf_1(\mathbf{X}) + C^2 f_2(\mathbf{X}) + \cdots + C^{\min(M,J)\cdot k} f_{\min(M,J)\cdot k}(\mathbf{X})\Big) \,, \end{aligned} \tag{8}$$

where $f_i(\mathbf{X})$ collects all products of $\delta(x_i - x_j)$ at the order of $C^i$. The first term in parenthesis corresponds to the noninteracting result, is analytically known and uninteresting. The interaction-induced part $\Delta Q_{MJ}$ is what we are looking for:

$$\begin{aligned} \Delta Q_{MJ} = \sum_{|\mathbf{P}\rangle,|\mathbf{X}\rangle} \mathrm{e}^{-\frac{\beta}{2m}(\boldsymbol{P_1^2}+\boldsymbol{P_2^2}+\cdots+\boldsymbol{P_k^2})} \langle \boldsymbol{P_1}|\boldsymbol{X_1}\rangle \langle \boldsymbol{X_1}|\boldsymbol{P_2}\rangle \langle \boldsymbol{P_2}|\boldsymbol{X_2}\rangle \langle \boldsymbol{X_2}|\boldsymbol{P_3}\rangle \cdots \langle \boldsymbol{P_k}|\boldsymbol{X_k}\rangle \langle \boldsymbol{X_k}|\boldsymbol{P_1}\rangle \\ \times \Big(Cf_1(\mathbf{X}) + C^2 f_2(\mathbf{X}) + \cdots + C^{\min(M,J)\cdot k} f_{\min(M,J)\cdot k}(\mathbf{X})\Big) \,. \end{aligned} \tag{9}$$

At each order in $C$, the summation is carried out over the coordinate variables first. In the continuum limit, the summation $\sum_x \mathrm{e}^{ix(p_i - p_j)}$ becomes the definition of a Dirac $\delta$-function (up to a constant prefactor) such that $\Delta Q_{MJ}$ takes the form

$$\Delta Q_{MJ} = \sum_{|\mathbf{P}\rangle} \mathrm{e}^{-\frac{\beta}{2m}(\boldsymbol{P_1^2}+\boldsymbol{P_2^2}+\cdots+\boldsymbol{P_k^2})} \Big(Cg_1(\mathbf{P}) + C^2 g_2(\mathbf{P}) + \cdots + C^{\min(M,J)\cdot k} g_{\min(M,J)\cdot k}(\mathbf{P})\Big) \,, \tag{10}$$

where $g_i(\mathbf{P})$ results from $f_i$ after the coordinate variables have been contracted, and is essentially a combination of Dirac $\delta$ functions in $\mathbf{P}$ encoding the dynamics and particle statistics (in our case fermionic). Contracting those $\delta$ functions with the propagator factor $\mathrm{e}^{-\frac{\beta}{2m}(\boldsymbol{P_1}^2+\boldsymbol{P_2}^2+\cdots+\boldsymbol{P_k}^2)}$, we finally obtain $\Delta Q_{MJ}$ which, in the continuum limit, takes the form of a combination of multi-dimensional Gaussian integrals in momentum space.

At a specific $C^i$ order, the evalutaion requires the explicit expansion of $2k$ Slater determinants, yielding $(M!N!)^{2k}$ terms multiplied by a combinatorial factor from $f_i$. Taking into account symmetries in the product of Slater determinants, the effective number of terms that need to be evaluated can be halved to $(M!N!)^k$ and the cyclic symmetry can further reduce the number by $1/k$. The evaluation is made possible by custom-made codes that carry out the algebra manipulations automatically. The codes are scalable and can be easily adapted to large-scale parallel deployment.

It may be possible to reduce the effective number of terms even further. We leave those investigations to future work as it may help to conduct the calculation at higher $k$ and $\Delta b_n$. Based on the above, we comment on the possibility of extending our calculations beyond $\Delta b_5$. While it is possible to push our method up to $k = 3$ for $\Delta b_6$ and $k = 2$ for $\Delta b_7$, such limited results do not provide enough information to carry out a reliable extrapolation to the large-$k$ limit. As the combined results presented here required $O(10^5)$ CPU hours, we estimate that a reliable determination of $\Delta b_6$ or $\Delta b_7$ would require more than $O(10^8)$ CPU hours and is therefore beyond the reach of our current computational resources. However, those calculations may be within the reach of supercomputers, especially if combined with aggressive code optimizations. Extending our work beyond beyond the unitary limit is also possible, but not without incurring much larger uncertainties than the ones shown in the main text. As shown there, the relative errors in our determination of the third to fifth coefficients at unitarity are roughly 1%, 3%, and 8%, respectively.

## II. RENORMALIZATION

As mentioned in the main text, we carry out two different renormalization procedures which, in the limit of a continuous temporal lattice (i.e. large $k$ in the Trotter-Suzuki factorization) should yield the same result. In both cases, a spatial lattice is used as a regulator and is quickly eliminated when the intermediate momentum sums appearing in the calculation (see previous section) are evaluated as infinite integrals. In the process, the dependence on the bare coupling is tuned as follows.

*Procedure I.-* Here, we tune the bare coupling such that the calculation of $\Delta b_2$, at a given order $k$ in the Trotter-Suzuki factorization, reproduces the known, continuum-limit value of that coefficient, which at unitarity is simply $\Delta b_2^{\mathrm{UFG}} = 1/\sqrt{2}$. The idea of this procedure is that one is approaching the continuum limit along the 'line of constant physics', where the physics is set by the second-order virial coefficient. More specifically, our calculations yield, at a given $k$, analytic expressions for $\Delta b_n$ which are polynomials in the dimensionless coupling $\tilde{C} = C/\lambda_T^d$, where $C = e^{\beta g/k} - 1$ (see also previous section). The latter is then determined by matching to $\Delta b_2$. The remaining $\Delta b_n$ are then simply evaluated by plugging in the tuned value of $\tilde{C}$.

*Procedure II.-* In this case, which we implemented only at the strongest coupling we explored, namely the unitary limit, we tuned the bare coupling such that the largest eigenvalue of the factorized transfer matrix matched the value dictated by Lüscher's formula. As we show next, this can be accomplished mostly analytically. The Trotter-Suzuki-factorized transfer matrix is

$$\mathcal{T}_k \equiv e^{-\beta\hat{T}/(2k)} e^{-\beta\hat{V}/k} e^{-\beta\hat{T}/(2k)}, \tag{11}$$

whose two-body matrix elements, in the center-of-mass frame, are given by

$$T(\boldsymbol{p_r}, \boldsymbol{q_r}) = \langle \boldsymbol{p_1}\boldsymbol{p_2}| \mathrm{e}^{-\beta\hat{T}/(2k)} \mathrm{e}^{-\beta\hat{V}/k} \mathrm{e}^{-\beta\hat{T}/(2k)} |\boldsymbol{q_1}\boldsymbol{q_2}\rangle \,, \tag{12}$$

where

$$\begin{cases} \boldsymbol{p_1} + \boldsymbol{p_2} = 0 \\ \boldsymbol{q_1} + \boldsymbol{q_2} = 0 \end{cases} \quad \text{and} \quad \begin{cases} \boldsymbol{p_1} - \boldsymbol{p_2} = 2\boldsymbol{p_r} \\ \boldsymbol{q_1} - \boldsymbol{q_2} = 2\boldsymbol{q_r} \end{cases}. \tag{13}$$

Inserting complete sets of states as advocated in the previous section and using Eq. (7), we have

$$T(\boldsymbol{p_r}, \boldsymbol{q_r}) = \mathrm{e}^{-\beta p_r^2/(2k)} \mathrm{e}^{-\beta q_r^2/(2k)} \left( \delta_{\boldsymbol{p_r}\boldsymbol{q_r}} + \frac{C}{V} \right), \tag{14}$$

which evaluated at momenta $\boldsymbol{p_r} = 2\pi\boldsymbol{a}/L$ and $\boldsymbol{q_r} = 2\pi\boldsymbol{b}/L$, where $\boldsymbol{a}$ and $\boldsymbol{b}$ are integer vectors, becomes

$$T_{\boldsymbol{ab}} = f_{\boldsymbol{a}} f_{\boldsymbol{b}} \left( \delta_{\boldsymbol{ab}} + \frac{C}{V} \right) \equiv f_{\boldsymbol{a}} f_{\boldsymbol{b}} \left[ \delta_{\boldsymbol{ab}} + \tilde{C}\,(2\pi x)^{3/2} \right]. \tag{15}$$

For convenience, we defined $f_{\boldsymbol{a}} = \exp\left(-\frac{x}{2k}\frac{4\pi^2\boldsymbol{a}^2}{m}\right)$, rescale $C$ into $\tilde{C}$, and used $x = \beta/L^2$. Tuning $\tilde{C}$ to reproduce the leading eigenvalue $\lambda_0 = \exp\left(-\frac{x}{k}\frac{4\pi^2\eta_0^2}{m}\right)$ amounts to imposing the condition

$$\sum_{\mathbf{b}} [T - \lambda_0 I]_{\mathbf{ab}}\, \mathbf{v_b} = 0, \tag{16}$$

which can be solved analytically to obtain the dependence of the bare coupling on $\lambda_0$:

$$\tilde{C} = \frac{1}{(2\pi x)^{\frac{3}{2}}}\left[\sum_{\boldsymbol{a}}^{\Lambda} \frac{1}{\lambda_0/f_{\boldsymbol{a}}^2 - 1}\right]^{-1}, \tag{17}$$

which becomes Eq. (12) in the main text in the limit $\Lambda \to \infty$.

As a way to compare the two renormalization procedures, we construct the transfer matrix using the coupling obtained with the first procedure, i.e. the renormalized $\tilde{C}$ tuned to $\Delta b_2^{\mathrm{UFG}}$. The largest eigenvalue $\bar{\lambda}_0$ of that matrix is then compared with the value $\lambda_0$ dictated by Lüscher's formula, as shown in Fig. 1. There, we plot the ratio $\bar{\lambda}_0/\lambda_0$ as a function of $1/k$ at different values of $x$. As noted in the main text, the continuum limit is approached as $x \ll 1$. As $k$ increases and $x$ decreases, Fig. 1 shows that our first renormalization procedure approaches the correct limiting value.

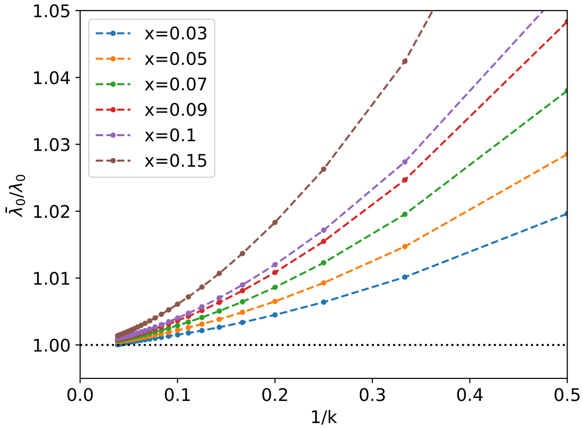


FIG. 1. The ratio between the largest eigenvalue $\bar{\lambda}_0$ of transfer matrix obtained for $\tilde{C}$ tuned to $\Delta b_2^{\mathrm{UFG}}$ and the one corresponding to Lüscher's formula $\lambda_0$, as functions of the discretization order $k$, shown as $1/k$, for several values of the parameter $x = \beta/L^2$.

## III. EXTRAPOLATION TO THE LARGE-$k$ LIMIT AND RESULTING UNCERTAINTY

Our calculations of $\Delta b_n$ using the Trotter-Suzuki factorization yield results with a smooth dependence on $k$, which must be captured in order to extrapolate to the large-$k$ limit. Different $\Delta b_n$ present similarities as well as differences in their behavior as a function of $k$. As an example, the $k$ dependence of $\Delta b_4$ and $\Delta b_5$ is shown in Fig. 2.

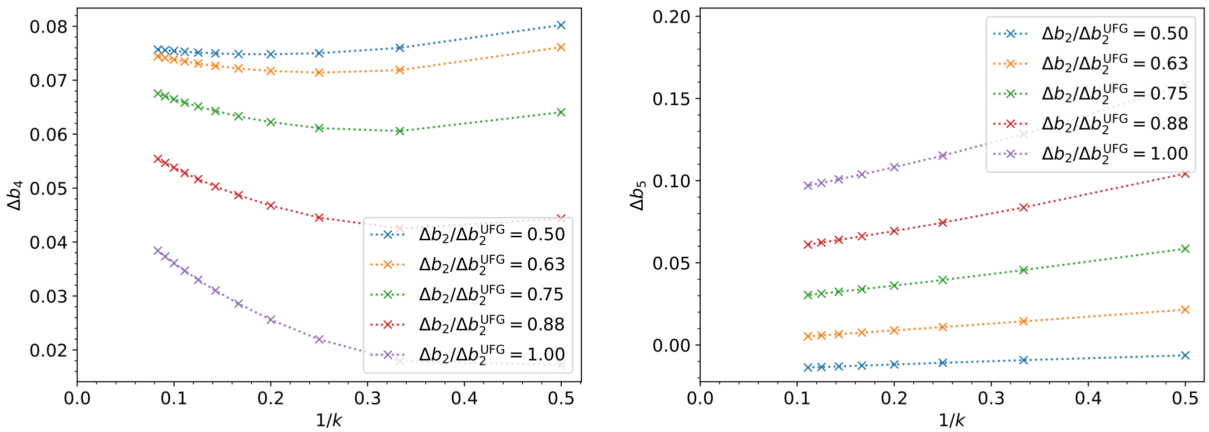


FIG. 2. Our results for $\Delta b_4$ (left) and $\Delta b_5$ (right) as functions of $1/k$ for several values of the coupling, parametrized by $\Delta b_2/\Delta b_2^{\rm UFG}$ as in the main text.

To extrapolate to the large-$k$ limit given limited information (namely up to $k = 21$ for $\Delta b_3$, $k = 12$ for $\Delta b_4$, and $k = 9$ for $\Delta b_5$), one can always attempt to do so directly using the plots of Fig. 2, but we found that approach to be too subjective and not easy to apply consistently across the $\Delta b_n$ we studied. We determined that, instead, a more objective and consistent way to extrapolate (across all $\Delta b_n$ we studied) is as described below. We stress, however, that no extrapolation scheme or analysis is better than more data, i.e. calculations at higher $k$. It should therefore be borne in mind that the final central values and uncertainties we quote in the main text should always be considered as tied to the amount of information analyzed (i.e. the various orders we computed). Future analyses and computational optimizations may very well be able to improve our estimates or provide more confidence on our present results.

To understand our extrapolation scheme, note that each $\Delta b_n$ depends on the dimensionless parameter $\tilde{C}$ (as explained in Sec. I) and that that dependence varies as $k$ is increased: more terms are added to the formula for $\Delta b_n$ with higher powers of $\tilde{C}$ and the prefactors of extant terms change as well. To obtain the uncertainty in a given $\Delta b_n$, we study the lines of constant $\Delta b_n$ as a function of $\tilde{C}$ and $k$. A given value of $\Delta b_n$ determines one such line $\tilde{C}_{\Delta b_n}(k)$. Since we use $\Delta b_2$ to renormalize, that determines a target value $\tilde{C}_{\Delta b_2}(k)$. We are therefore interested in the curves $\tilde{C}_{\Delta b_n}(k)/\tilde{C}_{\Delta b_2}(k)$ and where they cross unity for various possible values of $\Delta b_n$. We show an example of such curves in Fig. 3.

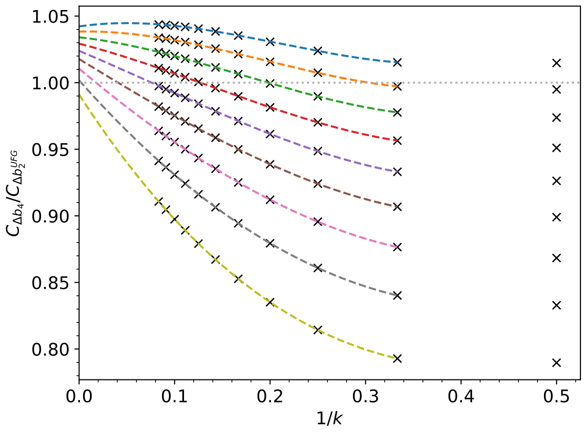


FIG. 3. $\tilde{C}/\tilde{C}_{\Delta b_2}$ as a function of $1/k$, at several fixed values of $\Delta b_4$. The crosses show the various orders $k$ calculated. The dashed lines show our polynomial fit and extrapolation to large $k$. The dashed-line endpoints at $k = 3$ indicate that data below that value of $k$ was not included in the fit. The same criterion was applied to our analyses of $\Delta b_3$ and $\Delta b_5$.

As shown in the example of Fig. 3, we analyze our data for $\tilde{C}_{\Delta b_n}(k)/\tilde{C}_{\Delta b_2}(k)$ as a function of $1/k$ using a polynomial

fit, with which we extrapolate to the large-$k$ limit. Here, different fits can lead to a spread of results when analyzing the locations at which the various extrapolations cross unity. Such crossings are shown in Fig. 4, which displays the case of $\Delta b_4$ (left) and $\Delta b_5$ (right) in the unitary limit. The variation in the crossings determines the uncertainty in the results quoted in the main text.

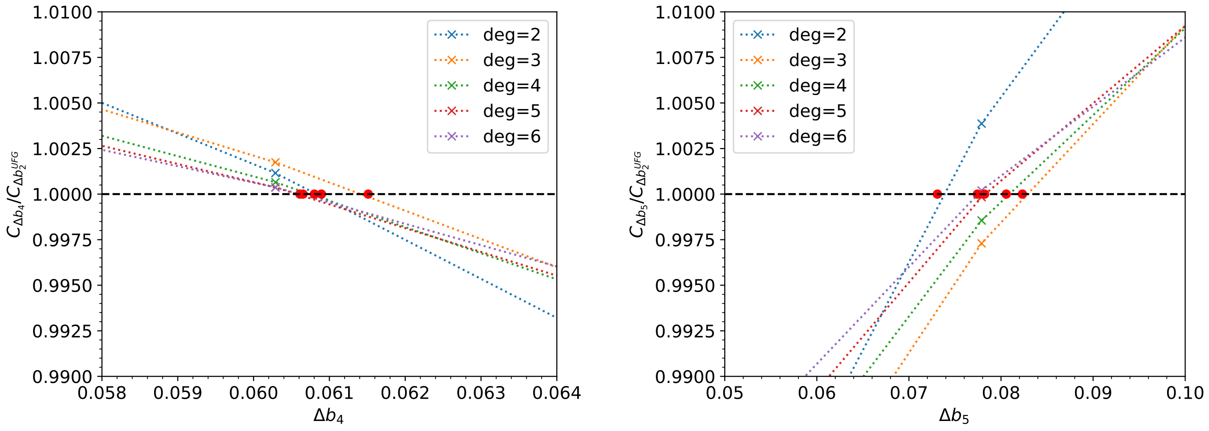


FIG. 4. Uncertainty estimation from polynomial fits at different degrees for $\Delta b_4$ (left) and $\Delta b_5$(right) in the unitary limit.

## IV. COMPARISON OF $\Delta b_2$ AND TRANSFER-MATRIX RENORMALIZATION PROCEDURES.

As mentioned above and in the main text, we pursued two different renormalization procedures when studying the unitary limit. In this section we show a comparison of these procedures. For the transfer-matrix renormalization (procedure II in the main text) we explored several values of the parameter $x = \beta/L^2$ (see above and main text). As $x \to 0$, we approach the continuum limit, where we expect the results of both of procedures to be consistent with each other.

In Fig. 5 (left) we show a calculation of $\Delta b_2$ at unitarity using our renormalization procedure II and the extrapolation scheme explained in the previous section. As $x \to 0$, we find that $\Delta b_2$ differs from its expected value by less than 0.25%. In the same figure (right) we show the corresponding results for $\Delta b_3$ and compare them with our renormalization procedure I. We find that the results of both procedures are consistent with each other within the uncertainties.

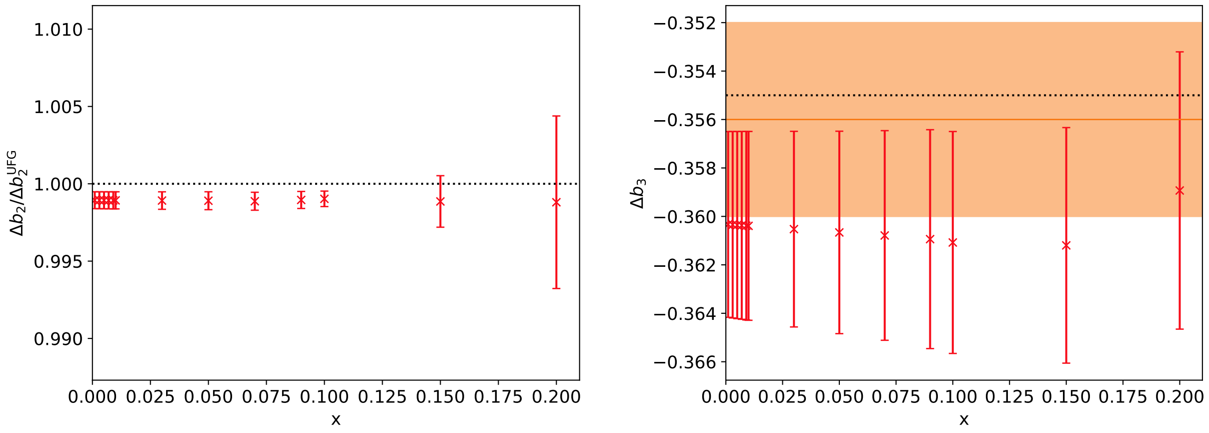


FIG. 5. **Left**: Results for $\Delta b_2$ (red error bars) at unitarity using our renormalization procedure II and the extrapolation scheme explained in the previous section, as a function of $x$. **Right**: Same as left but for $\Delta b_3$ (red error bars) compared with our renormalization procedure I (orange error band); the dotted line shows $\Delta b_3 = 0.3551$ (note that the entire vertical scale in this plot covers a range that is about 4% of the expected value).

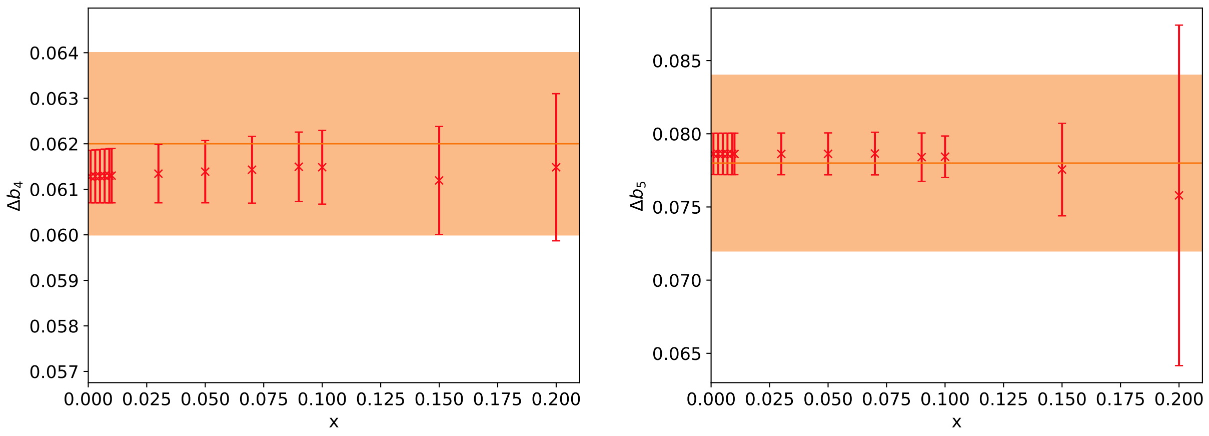


FIG. 6. **Left**: Results for $\Delta b_4$ (red error bars) at unitarity using our renormalization procedure II and the extrapolation scheme explained in the previous section, as a function of $x$, compared with our renormalization procedure I (orange error band). **Right**: Same as left but for $\Delta b_5$. Note: the entire vertical scales in these plots cover ranges of 11% (left) and 30% (right) of the final reported values of $\Delta b_4$ and $\Delta b_5$, respectively.

## V. DERIVATION OF POLARIZED VIRIAL COEFFICIENTS $\Delta b_{mj}$

Similar to Eq. (4) and Eq. (5) in the main text, the grand-canonical partition function for a polarized system is given by

$$\mathcal{Z} = \sum_{N=0}^{\infty} \sum_{\substack{M,J>0 \\ M+J=N}} z_{\uparrow}^{M} z_{\downarrow}^{J} Q_{MJ}, \tag{18}$$

where $z_s$ is the fugacity for species $s$ and $Q_{MJ}$ is the canonical partition function for $M$ particles of spin-$\uparrow$ and $J$ particles of spin-$\downarrow$. The polarized virial coefficients $\Delta b_{mj}$ are defined through

$$\ln(\mathcal{Z}/\mathcal{Z}_0) = Q_1 \sum_{n=2}^{\infty} \sum_{\substack{m,j>0 \\ m+j=n}} \Delta b_{mj} z_{\uparrow}^{m} z_{\downarrow}^{j}, \tag{19}$$

where $b_{mj} = b_{jm}$ for the mass-balanced case and $Q_1 = 2Q_{10}$ is the single-particle partition function. Expanding the logarithm of Eq. (18) in powers of $z_\uparrow$ and $z_\downarrow$, one obtains the explicit form of $\Delta b_{mj}$ in terms of the $Q_{MJ}$. For example,

$$\begin{aligned} \Delta b_{31} &= \frac{\Delta Q_{31}}{Q_1} - \frac{Q_{10}^2 - Q_{10}(2\beta)}{4Q_{10}} \Delta Q_{11} - \frac{1}{2}\Delta Q_{21} + \frac{Q_{10}}{2}\Delta Q_{11} \\ \Delta b_{22} &= \frac{\Delta Q_{22}}{Q_1} - \frac{\Delta Q_{11}^2}{4Q_{10}} - \frac{Q_{10}}{2}\Delta Q_{11} - \Delta Q_{21} + Q_{10}\Delta Q_{11} \end{aligned} \tag{20}$$

where $\Delta Q_{MJ}$ indicates the change in $Q_{MJ}$ due to interactions. In the above two expressions and their higher-order counterparts used in this work, all the contributions to the final results are actually contained in the first term on the right-hand side. Every term beyond the first one cancels out against identical contributions present in the first term. These cancellations provide crucial tests as the terms being cancelled scale as a positive power of the volume $V$, whereas the final result must be volume-independent.

## VI. APPLICATIONS

In this section we present a few comparisons of our results for the virial expansion with experimentally measurable (and measured) quantities.

### A. Tan's contact of spin-balanced system

Tan's contact can be obtained via the so-called adiabatic relation, differentiating with respect to the coupling $\lambda$. Since our estimates of $\Delta b_n$ use $\Delta b_2$ as our physical dimensionless coupling, we use the chain rule when differentiating $\Delta\Omega$:

$$\mathcal{I} = -\frac{4\pi}{\beta}\frac{\partial(\beta\Omega)}{\partial a_0^{-1}} = \frac{4\pi}{\sqrt{\beta}}\frac{\partial \ln \mathcal{Z}}{\partial \Delta b_2}\frac{\partial \Delta b_2}{\partial \lambda}, \tag{21}$$

where $\lambda = \sqrt{\beta}/a_0$ as in the main text. Thus,

$$\mathcal{I} = \frac{4\pi}{\beta} Q_1 \lambda_T \sum_{m=2}^{\infty} c_m z^m, \tag{22}$$

where $\lambda_T = \sqrt{2\pi\beta}$ and

$$c_m = \frac{1}{\sqrt{2\pi}}\frac{\partial \Delta b_m}{\partial \Delta b_2}\frac{\partial \Delta b_2}{\partial \lambda}, \tag{23}$$

where the Beth-Uhlenbeck formula yields

$$\frac{\partial \Delta b_2}{\partial \lambda} = \sqrt{\frac{2}{\pi}} + \sqrt{2}\,\lambda\, e^{\lambda^2}(1+\mathrm{erf}(\lambda)). \tag{24}$$

While $c_2$ is thus fully determined by the Beth-Uhlenbeck formula, we also provide here estimates of $c_3$, $c_4$, and $c_5$, shown in Fig. 7 (left).

In our Fig. 7 (right), we display the manifestly dimensionless, thermodynamically intensive form

$$\frac{\mathcal{I}}{N k_F} = 3\pi^2(4\pi)^2 \frac{1}{k_F^4 \lambda_T^4}\sum_{m=2}^{\infty} c_m z^m = 3\pi^2\left(\frac{T}{T_F}\right)^2 \sum_{m=2}^{\infty} c_m z^m, \tag{25}$$

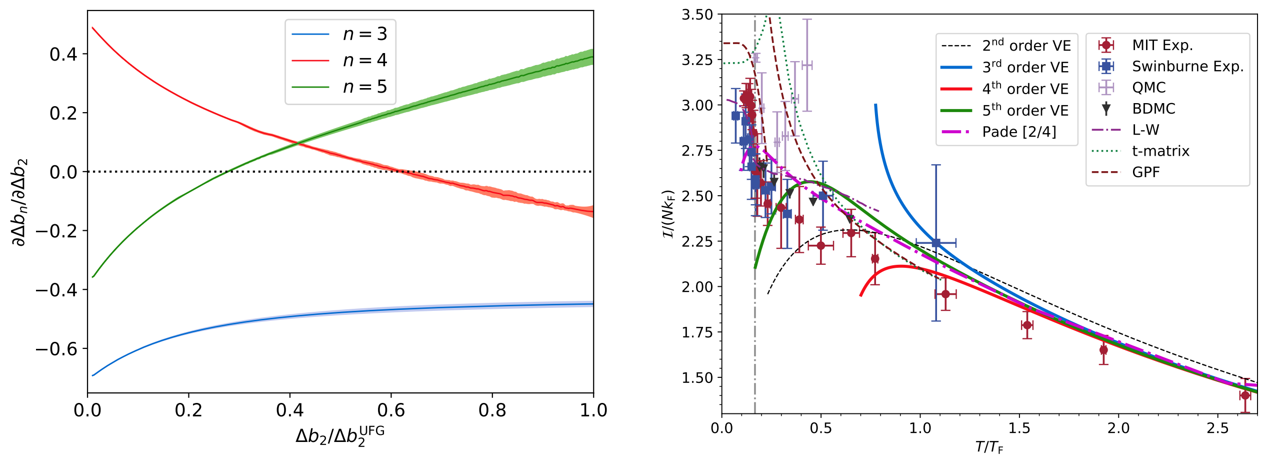


FIG. 7. **Left**: Derivative of $\Delta b_n$ with respect to $\Delta b_2$ as a function of the coupling. **Right**: Dimensionless contact $\mathcal{I}/(N k_F)$ as a function of the dimensionless temperature $T/T_F$. Our virial expansion results at different orders are shown as thick solid line in blue (3$^{\rm rd}$ order), red (4$^{\rm th}$ order), and green (5$^{\rm th}$ order). The solid purple line is the result using Padé approximant at order [2/4] on the sum series to fifth order (see Sec. VII for details). The gray dashed line shows the critical temperature $T_c/T_F = 0.167$. Also shown are the experimental measurements from Ref. [1] (dark red data with error bars); the experimental measurements from Ref. [2] (dark blue squares); the Quantum Monte Carlo (QMC) estimates from Ref. [3] (light purple plus signs); the bold-diagrammatic QMC estimates from Ref. [4] (gray triangles); the Luttinger-Ward (LW) results from Ref. [5] (purple dash-dot line); the T-Matrix calculation from Ref. [6] (green dotted line); and the Gaussian-pair-fluctuation theory (GPF) estimates from Ref. [7] (dark red dashed line).

where we used $Q_1 = 2V/\lambda_T^3$, $k_F^3 = 3\pi^2 n$ and $n = N/V$ in the first identity, and $T_F = k_F^2/2$ and $T = 2\pi/\lambda_T^2$ in the second identity. The dimensionless temperature $T/T_F$ is related to the per-species dimensionless density $\rho$ by $\rho \equiv \lambda_T^3 n/2 = 4/(3\sqrt{\pi})(T_F/T)^{3/2}$ and $\rho$ is given in the virial expansion by

$$\rho = \rho_0 + \sum_{m=2}^{\infty} m\Delta b_m z^m, \tag{26}$$

where $\rho_0$ is the dimensionless density of non-interacting Fermi gas, i.e.

$$\rho_0 = f_{3/2}(z) = \frac{4}{\sqrt{\pi}} \int_0^\infty \mathrm{d}x \frac{ze^{-x^2}}{1+ze^{-x^2}}, \tag{27}$$

where $f_{3/2}(z) = \mathrm{Li}_{3/2}(-z)$ is the Fermi-Dirac function, which is given by the polylogarithm function $\mathrm{Li}_s(x)$. Therefore, for a given fugacity, we first calculate $T/T_F$ through the density $n$, and then the contact using Eq. (25).

### B. Tan's contact of spin-imbalanced system

In spin imbalanced systems, the difference in chemical potential will lead to a different density for each flavor. By convention, we choose the majority (minority) type as spin-$\uparrow$ (spin-$\downarrow$) and define the impurity concentration as $n_\downarrow/n_\uparrow$. Similar to the spin-balanced case, the contact is given by

$$\mathcal{I} = \frac{4\pi}{\beta} Q_1 \lambda_T \sum_{m=2}^{\infty} \sum_{\substack{i,j>0 \\ i+j=m}} c_{ij} z_\uparrow^i z_\downarrow^j, \tag{28}$$

where $c_{ij}$ is

$$c_{ij} = \frac{1}{\sqrt{2\pi}} \frac{\partial \Delta b_{ij}}{\partial \Delta b_{11}} \frac{\partial \Delta b_{11}}{\partial \lambda}, \tag{29}$$

which is related to $c_m$ via $c_m = \sum_{i=1}^{m-1} c_{i(m-i)}$. The dimensionless contact takes the form

$$\frac{\mathcal{I}}{2N_\downarrow k_{F\uparrow}} = 3\pi^2 \left(\frac{T}{T_{F\uparrow}}\right)^2 \left(\frac{n_\uparrow}{n_\downarrow}\right) \sum_{m=2}^{\infty} \sum_{\substack{i,j>0 \\ i+j=m}} c_{ij} z_\uparrow^i z_\downarrow^j. \tag{30}$$

where we used $k_{F\uparrow}^3 = 6\pi^2 n_\uparrow$. The dimensionless temperature $T/T_{F\uparrow}$ is related to the spin-$\uparrow$ dimensionless density $\rho_\uparrow$ by $\rho_\uparrow = \lambda_T^3 n_\uparrow = 4/(3\sqrt{\pi})(T_{F\uparrow}/T)^{3/2}$ and $\rho_\uparrow$ is given by

$$\rho_\uparrow = f_{3/2}(z_\uparrow) + 2\sum_{m=2}^{\infty} \sum_{\substack{i,j>0 \\ i+j=m}} i\, b_{ij} z_\uparrow^i z_\downarrow^j. \tag{31}$$

For completeness, we also show the expression for $\rho_\downarrow$ as

$$\rho_\downarrow = f_{3/2}(z_\downarrow) + 2\sum_{m=2}^{\infty} \sum_{\substack{i,j>0 \\ i+j=m}} j\, b_{ij} z_\uparrow^i z_\downarrow^j. \tag{32}$$

In practice, the impurity concentration is fixed and, for a given $z_\uparrow$, one can first solve for $z_\downarrow$ using the above equations and then calculate the dimensionless contact $\mathcal{I}/(2N_\downarrow k_{F\uparrow})$ and dimensionless temperature $T/T_{F\uparrow}$. In Fig. 8, we compare the result of virial expansion to experimental measurements with impurity concentration of 10%.

Finally, we note for future reference that, in the noninteracting limit,

$$\frac{\mathcal{I}}{2N_\downarrow k_{F\uparrow}} = 2^{3/2}\sqrt{\pi}\left(\sqrt{2}-1\right)\sqrt{\frac{T}{T_{F\uparrow}}} n_\uparrow \lambda_T^3. \tag{33}$$

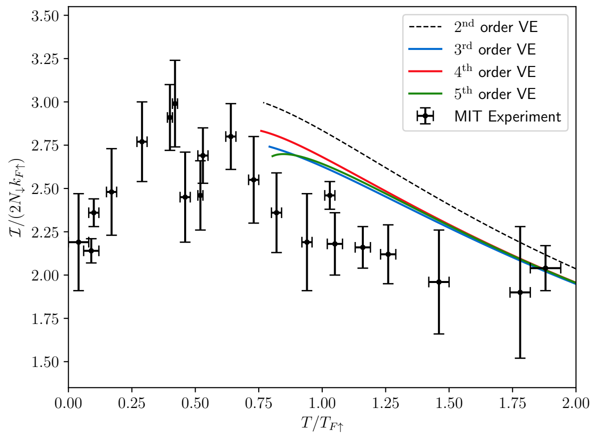


FIG. 8. The spin-imbalanced contact $\mathcal{I}/(N_\downarrow k_{F\uparrow})$ as a function of temperature $T_{F\uparrow}/T$. The black circles shows the experimental measurements from Ref. [8] at impurity concentration of 10%, the solid curves are the results of virial expansion.

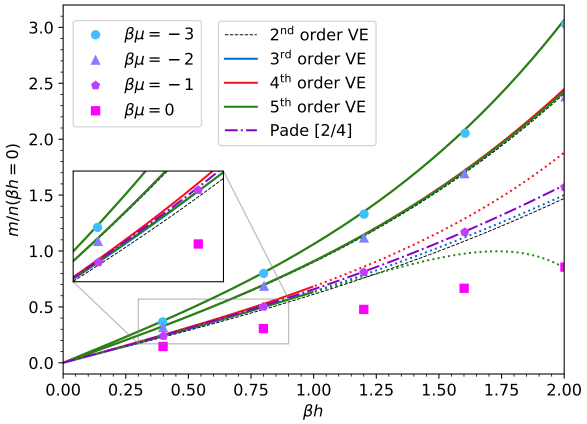


FIG. 9. Dimensionless magnetization $\bar{m} = m/n_0(\beta h = 0)$ as a function of dimensionless chemical potential difference $\beta h$. The circles ($\beta\mu$ = -3), triangles ($\beta\mu$ = -2), pentagons ($\beta\mu$ = -1) and squares ($\beta\mu$ = 0) are the QMC calculations from Ref. [9] for different values of $\beta\mu$. Note that only the results relevant to the virial expansion are presented here. The blue, red, and green curves show the result of virial expansion at third, fourth, and fifth order respectively. For $\beta\mu = -1$, part of the curve is shown as a dotted line to indicate the region where the virial expansion is not expected to be converge well, namely $z_\uparrow > 1$. The purple dash-dotted line is the Padé approximation at order [2/4] (see next section) for $\beta\mu = -1$, which shows better agreement with the QMC calculations than the finite-order virial expansion. The inset shows a closer view of the comparison between the virial expansion and QMC results, from which it is clear that the fifth-order virial expansion yields an improved estimate.

### C. Magnetization

In the case of polarized system, we define the dimensionless chemical potential $\beta\mu = \beta(\mu_\uparrow + \mu_\downarrow)/2$ and the dimensionless chemical potential difference $\beta h = \beta(\mu_\uparrow - \mu_\downarrow)/2$. Using Eq. (31) and Eq. (32), the dimensionless magnetization $\bar{m} = m/n_0(\beta h = 0)$, where $m = n_\uparrow - n_\downarrow$ is the magnetization, can be obtained by substituting in the fugacities $z_\uparrow = \exp(\beta\mu_\uparrow)$ and $z_\downarrow = \exp(\beta\mu_\downarrow)$ with $\mu_\uparrow = \mu + h$ and $\mu_\downarrow = \mu - h$. The result of $\bar{m}$ is shown as a function of $\beta h$ for $\beta\mu = -3, -2, -1$ and 0 in Fig. 9 and compared to a selection of QMC calculations from Ref. [9]. At $\beta\mu = -1$, due to the convergence issue of finite-order virial expansion for $\beta h > 1$, a Padé approximation at order [2/4] is also applied and find good agreement with previous findings.

## VII. RESUMMATION TECHNIQUES

For a given series $F(z)$ in form of

$$F(z) = \sum_n f_n z^n \tag{34}$$

the Padé approximation at $[M/N]$ order is given as

$$F(z) = \frac{P_M(z)}{Q_N(z)} = \frac{p_0 + p_1 z + \cdots + p_M z^M}{1 + q_1 z + \cdots + q_N z^N} \tag{35}$$

which often provides better approximation to the "infinite-order" results compared to the finite truncation.

In the case of the virial expansion, the finite-order series usually diverges for fugacities larger than unity and therefore fails at low temperature. Using the Padé approximation, one can then expect a better-behaved estimation in that regime. The work of Ref. [10] applied the Padé approximation to the third-order virial expansion for temperatures down to the superfluid phase and found agreement with experimental data with a maximum of 10% relative discrepancy. However, only the Padé approximant of order [1/1] was studied due to the limited access to higher-order virial coefficients. In Fig. 7 we show the result using a Padé approximant of order [2/4].

Another technique that can also enhance the convergence of a series at low temperature is Borel-Padé resummation, which combines the Borel integral sum with a Padé approximant. Given a divergent series $F(z)$ in the same form as in Eq. (34), applying the Borel transformation $\mathcal{B}$ generates a new series

$$\mathcal{B}F(z) = \sum_n \frac{f_n}{n!} z^n, \tag{36}$$

which usually converges better than the original one. The Borel integral sum of $F(z)$ is then given by

$$B(z) = \int_0^\infty \mathrm{d}t e^{-t} \mathcal{B}F(tz) \tag{37}$$

If the integral converges for the given $z$, we then have $F(z) = \sum_n f_n z^n = B(z)$. As the series is truncated at finite order, one can then apply the Padé approximation to the series $\mathcal{B}F(z) = P_M(z)/Q_N(z)$ and substitute it as the integrand, such that

$$B(z) = \int_0^\infty \mathrm{d}t e^{-t} \frac{P_M(tz)}{Q_N(tz)} \tag{38}$$

which defines the Borel-Padé resummation estimate.

As pointed out in Ref. [10], the validity of the Padé approximation cannot be taken for granted a priori as its form is not systematically controlled. Although there are successful applications of the Borel-Padé approximation in the field of QCD [11] and in cold atoms [12, 13], further investigations are still required for the virial expansion as it has different properties than those of perturbative expansions.

---


[1] M. J. H. Ku, A. T. Sommer, L. W. Cheuk, and M. W. Zwierlein, *Revealing the Superfluid Lambda Transition in the Universal Thermodynamics of a Unitary Fermi Gas*, Science **335**, 563 (2012).

[2] C. Carcy, S. Hoinka, M. G. Lingham, P. Dyke, C. C. N. Kuhn, H. Hu, and C. J. Vale, *Contact and sum rules in a near-uniform fermi gas at unitarity*, Phys. Rev. Lett. **122**, 203401 (2019).

[3] O. Goulko, and M. Wingate, *Numerical study of the unitary Fermi gas across the superfluid transition*, Phys. Rev. A **93**, 053604 (2016).

[4] R. Rossi, T. Ohgoe, E. Kozik, N. Prokof'ev, B. Svistunov, K. Van Houcke, and F. Werner, *Contact and Momentum Distribution of the Unitary Fermi Gas*, Phys. Rev. Lett. **121**, 130406 (2018).

[5] T. Enss, R. Haussmann, and W. Zwerger, *Viscosity and scale invariance in the unitary Fermi gas*, Ann. Phys. **326**, 770-796 (2011).

[6] F. Palestini, A. Perali, P. Pieri, and G. C. Strinati *Temperature and coupling dependence of the universal contact intensity for an ultracold Fermi gas*, Phys. Rev. A **82**, 021605 (2010).

[7] H. Hu, X.-J. Liu and P. D. Drummond *Universal contact of strongly interacting fermions at finite temperatures*, New J. Phys. **13**, 035007 (2011).

[8] Z. Yan, P. B. Patel, B. Mukherjee, R. J. Fletcher, J. Struck, and M. W. Zwierlein, *Boiling a Unitary Fermi Liquid*, Phys. Rev. Lett. **122**, 093401 (2019).

[9] L. Rammelmüller, A. C. Loheac, J. E. Drut, and J. Braun, *Finite-Temperature Equation of State of Polarized Fermions at Unitarity*, Phys. Rev. Lett. **121**, 173001 (2018).

[10] X.-J. Liu, *Virial expansion for a strongly correlated Fermi system and its application to ultracold atomic Fermi gases*, Phys. Rep. **524**, 37 (2013).

[11] M. Pindor, *Pade Approximants and Borel Summation for QCD Perturbation Expansions*, arXiv:hep-th/9903151.

[12] Y. Nishida and D. T. Son, *$\epsilon$ expansion for a Fermi Gas at Infinite Scattering Length*, Phys. Rev. Lett. **97**, 050403 (2006).

[13] P. Arnold, J. E. Drut, and D. T. Son, *Next-to-next-to-leading-order $\epsilon$ expansion for a Fermi gas at infinite scattering length*, Phys. Rev. A **75**, 043605 (2007).

TABLE I. Summary of estimations for $\Delta b_3$ to $\Delta b_5$ and their polarized componenets from weakly-coupling to the unitary limit

| $\Delta b_2/\Delta b_2^{\mathrm{UFG}}$ | $\Delta b_3$ | $\Delta b_{31}$ | $\Delta b_{22}$ | $\Delta b_4$ | $\Delta b_{41}$ | $\Delta b_{32}$ | $\Delta b_5$ |
|---|---|---|---|---|---|---|---|
| 0.01 | -0.0049522(3) | 0.0013460(1) | 0.0008380(1) | 0.0035300(4) | -0.0008741(1) | -0.00044537(7) | -0.0026389(4) |
| 0.04 | -0.018016(3) | 0.004881(1) | 0.0026880(9) | 0.012449(3) | -0.003168(1) | -0.0013243(4) | -0.008984(3) |
| 0.07 | -0.031612(9) | 0.008536(4) | 0.004052(1) | 0.021123(10) | -0.005537(3) | -0.0017921(6) | -0.014659(7) |
| 0.10 | -0.04464(1) | 0.012018(7) | 0.004816(2) | 0.02885(2) | -0.007793(5) | -0.0018236(1) | -0.01923(1) |
| 0.12 | -0.05615(3) | 0.015086(9) | 0.005052(3) | 0.03522(1) | -0.009777(8) | -0.0015190(3) | -0.02259(1) |
| 0.15 | -0.06832(5) | 0.01832(1) | 0.004848(7) | 0.04148(2) | -0.01187(1) | -0.000862(4) | -0.02546(3) |
| 0.18 | -0.08015(9) | 0.02145(1) | 0.004212(10) | 0.04710(2) | -0.01389(1) | 0.00009(1) | -0.02758(6) |
| 0.21 | -0.0917(1) | 0.02449(2) | 0.00318(2) | 0.05216(2) | -0.01585(2) | 0.00131(1) | -0.02908(5) |
| 0.24 | -0.1020(2) | 0.02722(2) | 0.00191(2) | 0.05634(2) | -0.01761(2) | 0.00265(2) | -0.02992(7) |
| 0.27 | -0.1131(3) | 0.03012(3) | 0.00019(3) | 0.06044(3) | -0.01948(3) | 0.00434(3) | -0.03029(9) |
| 0.30 | -0.1240(3) | 0.03299(3) | -0.00187(1) | 0.06411(4) | -0.02132(4) | 0.00625(4) | -0.0302(1) |
| 0.33 | -0.1347(4) | 0.03580(3) | -0.00432(8) | 0.06735(9) | -0.02313(5) | 0.00836(6) | -0.0295(2) |
| 0.36 | -0.1444(5) | 0.03834(4) | -0.00676(10) | 0.0699(1) | -0.02476(6) | 0.01047(7) | -0.0286(2) |
| 0.39 | -0.1549(6) | 0.04108(5) | -0.0097(1) | 0.0724(1) | -0.02652(8) | 0.01295(10) | -0.0271(3) |
| 0.42 | -0.1652(7) | 0.04379(6) | -0.0130(1) | 0.0746(2) | -0.02825(9) | 0.0156(1) | -0.0253(3) |
| 0.45 | -0.1755(9) | 0.04646(8) | -0.0165(1) | 0.0764(2) | -0.0300(1) | 0.0184(2) | -0.0231(4) |
| 0.47 | -0.1848(10) | 0.04888(9) | -0.0199(2) | 0.0778(2) | -0.0315(1) | 0.0212(2) | -0.0207(5) |
| 0.50 | -0.195(1) | 0.0515(1) | -0.0239(2) | 0.0791(3) | -0.0332(1) | 0.0243(3) | -0.0178(6) |
| 0.53 | -0.205(1) | 0.0541(1) | -0.0282(2) | 0.0800(3) | -0.0349(2) | 0.0276(4) | -0.0145(8) |
| 0.56 | -0.214(1) | 0.0565(2) | -0.0323(2) | 0.0806(4) | -0.0364(2) | 0.0308(4) | -0.0112(9) |
| 0.59 | -0.224(2) | 0.0590(2) | -0.0370(2) | 0.0810(4) | -0.0381(2) | 0.0344(5) | -0.007(1) |
| 0.62 | -0.234(2) | 0.0616(2) | -0.0420(3) | 0.0812(5) | -0.0397(2) | 0.0382(6) | -0.003(1) |
| 0.65 | -0.244(2) | 0.0641(2) | -0.0472(2) | 0.0811(5) | -0.0413(3) | 0.0421(7) | 0.002(2) |
| 0.68 | -0.253(2) | 0.0664(3) | -0.0522(3) | 0.0807(6) | -0.0428(3) | 0.0458(8) | 0.006(2) |
| 0.71 | -0.262(2) | 0.0689(3) | -0.0578(3) | 0.0801(7) | -0.0444(3) | 0.0500(10) | 0.011(2) |
| 0.74 | -0.272(2) | 0.0714(4) | -0.0636(3) | 0.0793(8) | -0.0460(4) | 0.054(1) | 0.017(2) |
| 0.77 | -0.282(3) | 0.0739(4) | -0.0697(3) | 0.0781(9) | -0.0476(4) | 0.059(1) | 0.022(3) |
| 0.79 | -0.290(3) | 0.0762(5) | -0.0754(4) | 0.0770(10) | -0.0491(4) | 0.063(1) | 0.028(3) |
| 0.82 | -0.300(3) | 0.0787(5) | -0.0819(5) | 0.075(1) | -0.0506(5) | 0.068(2) | 0.034(3) |
| 0.85 | -0.310(3) | 0.0811(5) | -0.0886(4) | 0.074(1) | -0.0522(5) | 0.073(2) | 0.041(4) |
| 0.88 | -0.319(3) | 0.0836(6) | -0.0955(5) | 0.072(1) | -0.0538(6) | 0.078(2) | 0.048(4) |
| 0.91 | -0.328(3) | 0.0858(7) | -0.1020(6) | 0.070(1) | -0.0552(6) | 0.082(2) | 0.055(5) |
| 0.94 | -0.337(4) | 0.0882(7) | -0.1092(6) | 0.067(2) | -0.0567(7) | 0.088(2) | 0.062(5) |
| 0.97 | -0.347(4) | 0.0907(8) | -0.1168(6) | 0.065(2) | -0.0583(7) | 0.093(3) | 0.070(5) |
| 1.00 | -0.356(4) | 0.0931(9) | -0.1244(7) | 0.062(2) | -0.0598(8) | 0.099(3) | 0.078(6) |
